# Supplementary material for: Context-Aware Visual Policy Network for Fine-Grained Image Captioning
Source: arXiv:1906.02365 source file (2019-06-06)
Supplement: Supplementary file 1 [file 7_appendix.tex]

\appendices
\section{Proof of the First Zonklar Equation}
Appendix one text goes here.

% you can choose not to have a title for an appendix
% if you want by leaving the argument blank
\section{}
Appendix two text goes here.
